# Supplementary material for: Calibration of a bumble bee foraging model using Approximate Bayesian Computation
Source: arXiv:2204.03287 source file (2022-10-26)
Supplement: Supplementary file 1 [file supplementary.pdf]

# Supplementary material
# Calibration of a pollination model using Approximate Bayesian Computation

Ullrika Sahlin

## 1 Simulation study

Table 1: *Proportion of datasets for which each approach failed. 'Rej': rejection ABC algorithm, 'LocNLH': local nonlinear heteroscedastic regression, 'ANLH': adaptive nonlinear heteroscedastic regression, 'RFA': adjusted random forest regression, 'wqRF' (resp; 'uwqRF'): weighted (resp. unweighted) quantile regression via random forests, 'qGBM L1' (resp; 'qGBM L2'): quantile regression via gradient boosting and $L_1$ (resp. $L_2$) loss. The percentages '2.5%' and '5%' correspond to the values of the threshold parameter $\varepsilon$*

| Method | $\tau_0$ | $f_0$ | $a$ | $b$ | $\beta_1$ | $\beta_2$ | $\beta_3$ | $\sigma^2$ |
|---|---|---|---|---|---|---|---|---|
| Rej 2.5% | 0.00 | 0.00 | 0.00 | 0.00 | 0.00 | 0.00 | 0.00 | 0.00 |
| Rej 5% | 0.00 | 0.00 | 0.00 | 0.00 | 0.00 | 0.00 | 0.00 | 0.00 |
| LocLH 2.5% | 0.30 | 0.25 | 0.25 | 0.27 | 0.26 | 0.23 | 0.27 | 0.25 |
| LocLH 5% | 0.19 | 0.19 | 0.21 | 0.27 | 0.14 | 0.20 | 0.16 | 0.16 |
| LocNLH 2.5% | 0.00 | 0.00 | 0.00 | 0.00 | 0.00 | 0.00 | 0.00 | 0.00 |
| LocNLH 5% | 0.00 | 0.00 | 0.00 | 0.00 | 0.00 | 0.00 | 0.00 | 0.00 |
| ANLH 2.5% | 0.00 | 0.00 | 0.00 | 0.00 | 0.00 | 0.00 | 0.00 | 0.00 |
| ANLH 5% | 0.00 | 0.00 | 0.00 | 0.00 | 0.00 | 0.00 | 0.00 | 0.00 |
| uwqRF | 0.00 | 0.00 | 0.00 | 0.00 | 0.00 | 0.00 | 0.00 | 0.00 |
| wqRF | 0.00 | 0.00 | 0.00 | 0.00 | 0.00 | 0.00 | 0.00 | 0.00 |
| RFA | 0.00 | 0.00 | 0.00 | 0.00 | 0.00 | 0.00 | 0.00 | 0.00 |
| qGBM L1 | 0.02 | 0.02 | 0.02 | 0.03 | 0.03 | 0.02 | 0.02 | 0.03 |
| qGBM L2 | 0.05 | 0.05 | 0.05 | 0.05 | 0.05 | 0.05 | 0.05 | 0.05 |

The following graphs represent the ABC posterior median versus the true parameter value that was used to generate the 100 simulated datasets in the simulation study.

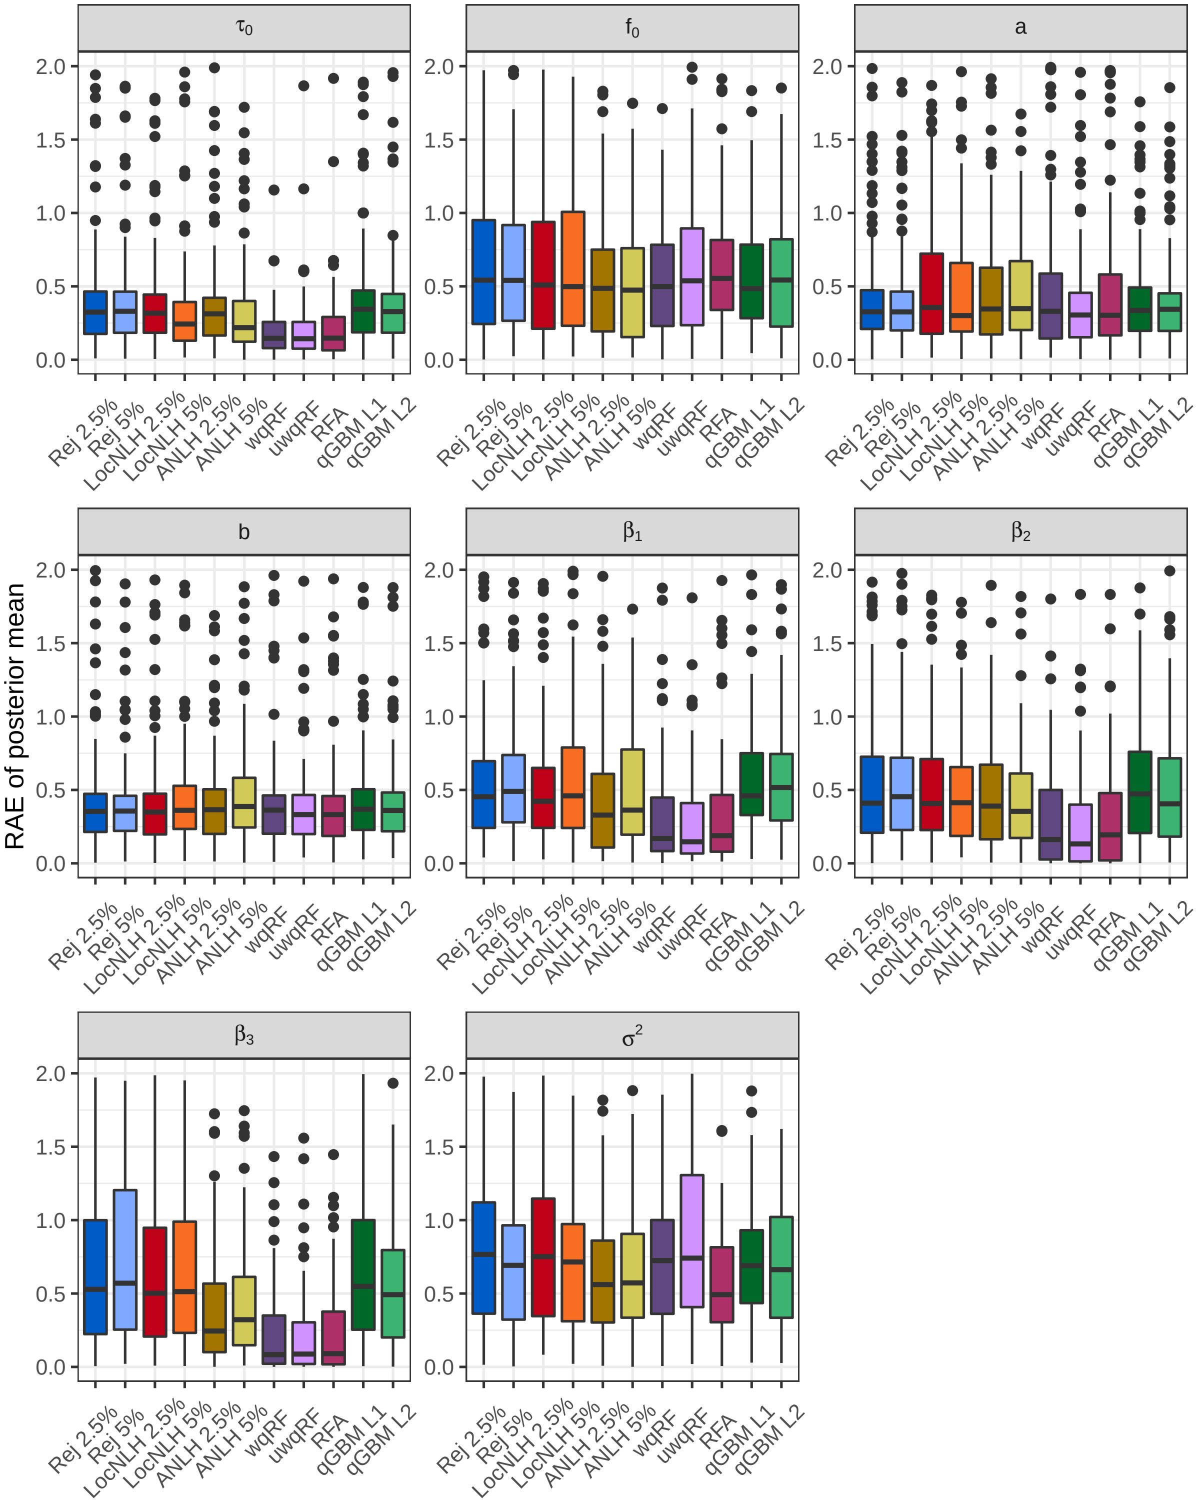


Figure 1: *Relative absolute error (RAE) of the posterior mean. The y-axes were truncated to 2 to make the plots clearer by removing some extreme points. 'Rej': rejection ABC algorithm, 'LocNLH': local nonlinear heteroscedastic regression, 'ANLH': adaptive nonlinear heteroscedastic regression, 'wqRF' (resp; 'uwqRF') : weighted (resp. unweighted) quantile regression via random forests, 'qGBM L1' (resp; 'qGBM L2'): quantile regression via gradient boosting and* $L_1$ *(resp.* $L_2$*) loss. The percentages '2.5%' and '5%' correspond to the values of the threshold parameter* $\varepsilon$

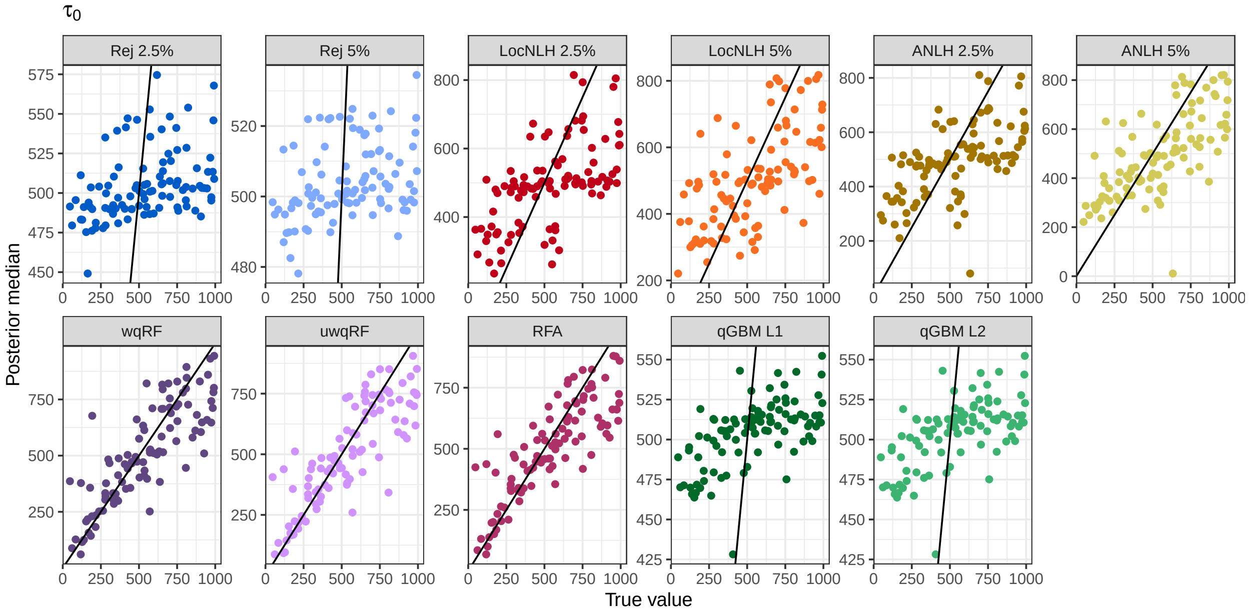


(a) $\tau_0$

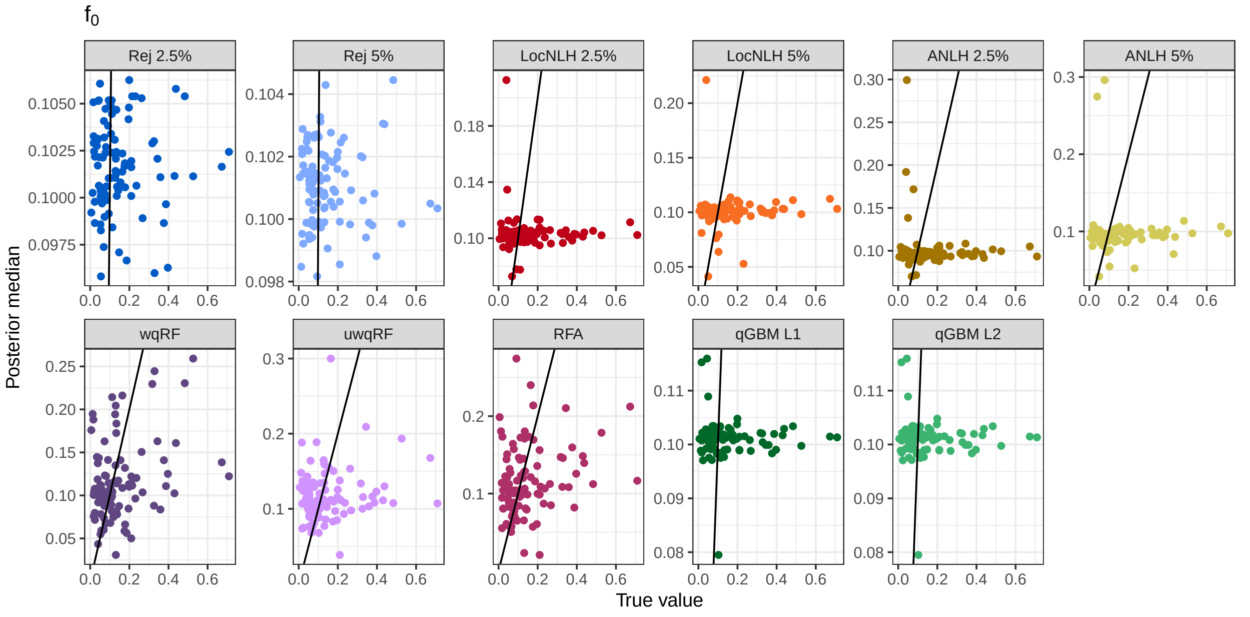


(b) $f_0$

Figure 2: *ABC posterior median as a function of the true parameter value. 'Rej': rejection ABC algorithm, 'LocNLH': local nonlinear heteroscedastic regression, 'ANLH': adaptive nonlinear heteroscedastic regression, 'RFA': adjusted random forest regression, 'wqRF' (resp; 'uwqRF') : weighted (resp. unweighted) quantile regression via random forests, 'qGBM L1' (resp; 'qGBM L2'): quantile regression via gradient boosting and $L_1$ (resp. $L_2$) loss. The percentages '2.5%' and '5%' correspond to the values of the threshold parameter $\varepsilon$*

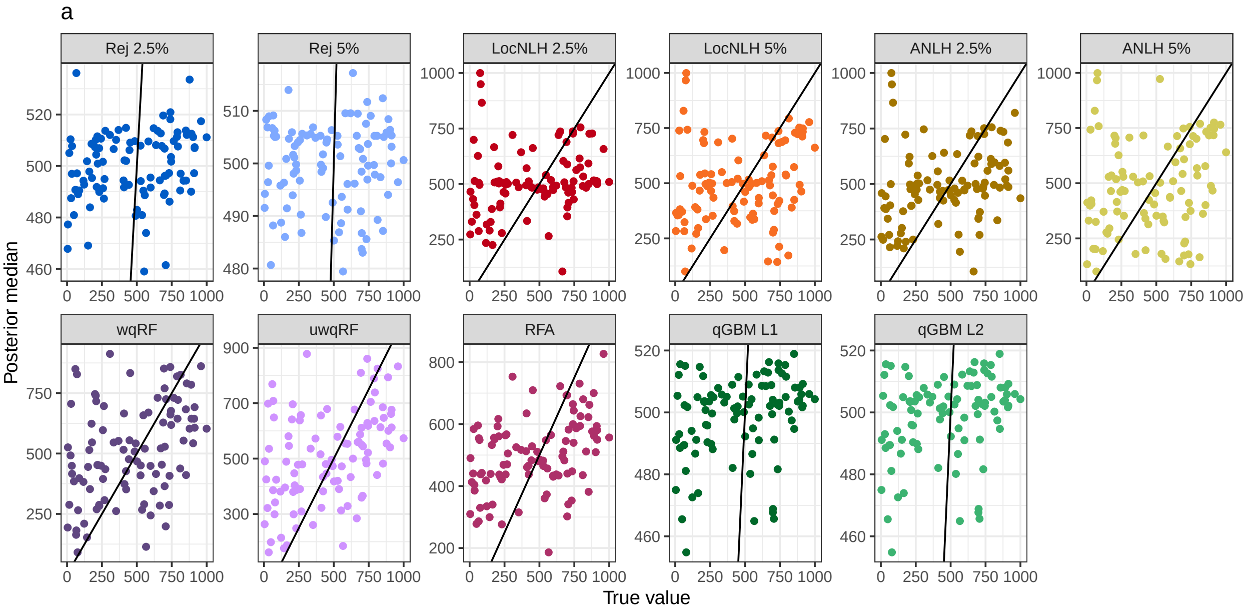


(c) $a$

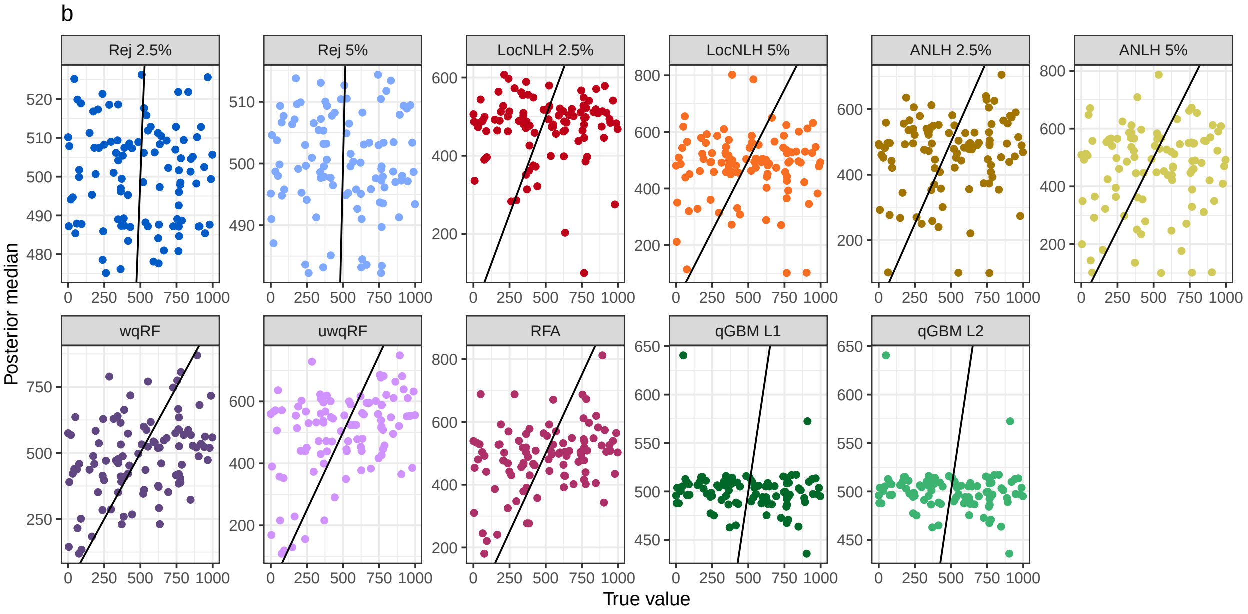


(d) $b$

Figure 2: *ABC posterior median as a function of the true parameter value (cont.). 'Rej': rejection ABC algorithm, 'LocNLH': local nonlinear heteroscedastic regression, 'ANLH': adaptive nonlinear heteroscedastic regression, 'RFA': adjusted random forest regression, 'wqRF' (resp; 'uwqRF') : weighted (resp. unweighted) quantile regression via random forests, 'qGBM L1' (resp; 'qGBM L2'): quantile regression via gradient boosting and* $L_1$ *(resp.* $L_2$*) loss. The percentages '2.5%' and '5%' correspond to the values of the threshold parameter* $\varepsilon$

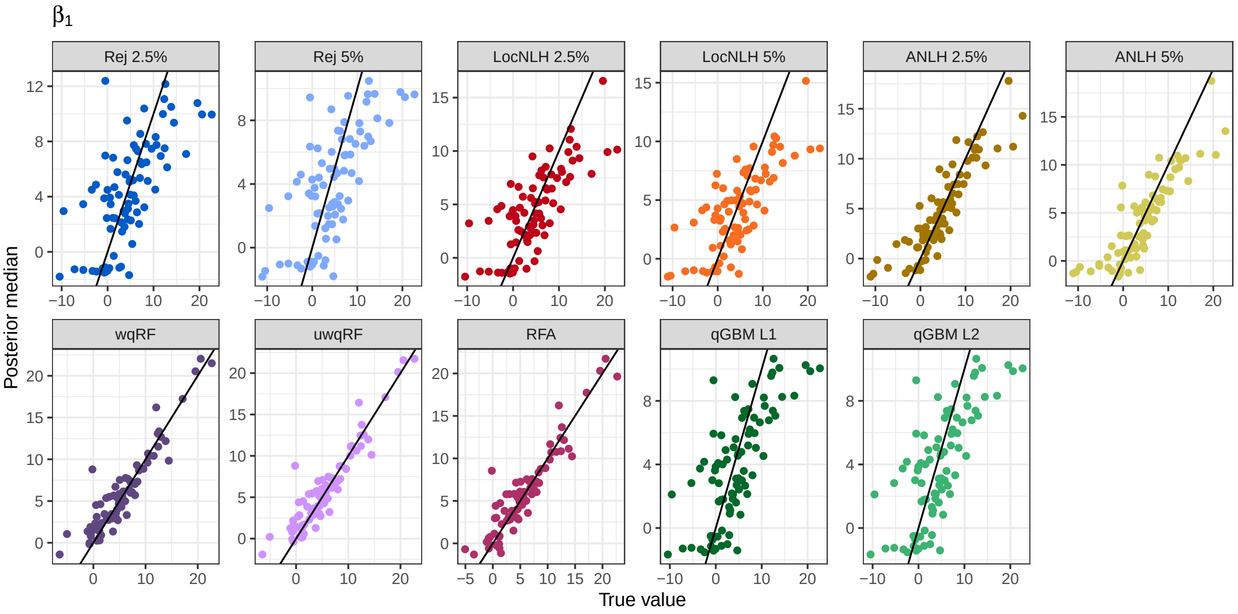


(e) $\beta_1$

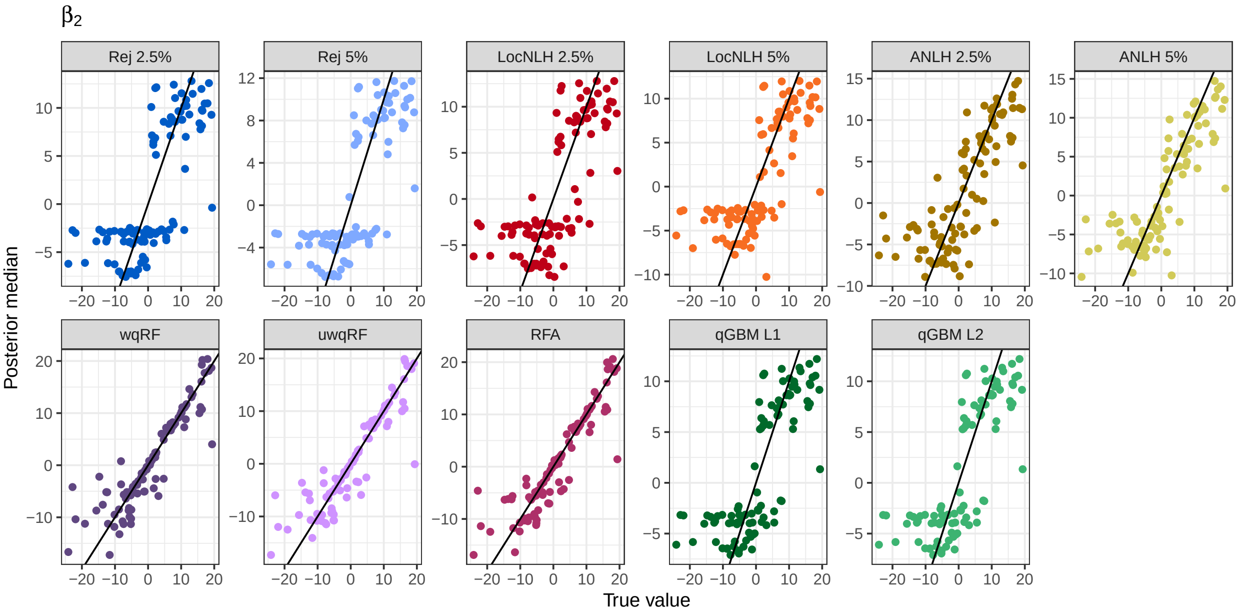


(f) $\beta_2$

Figure 2: *ABC posterior median as a function of the true parameter value (cont.). 'Rej': rejection ABC algorithm, 'LocNLH': local nonlinear heteroscedastic regression, 'ANLH': adaptive nonlinear heteroscedastic regression, 'RFA': adjusted random forest regression, 'wqRF' (resp; 'uwqRF') : weighted (resp. unweighted) quantile regression via random forests, 'qGBM L1' (resp; 'qGBM L2'): quantile regression via gradient boosting and $L_1$ (resp. $L_2$) loss. The percentages '2.5%' and '5%' correspond to the values of the threshold parameter $\varepsilon$*

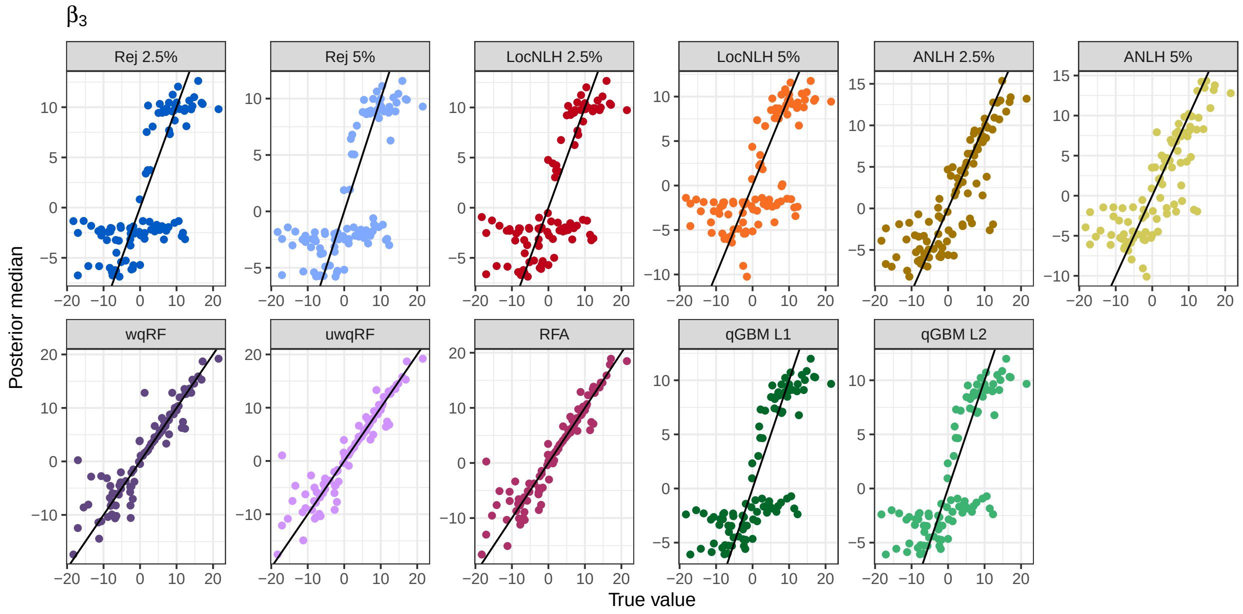


(g) $\beta_3$

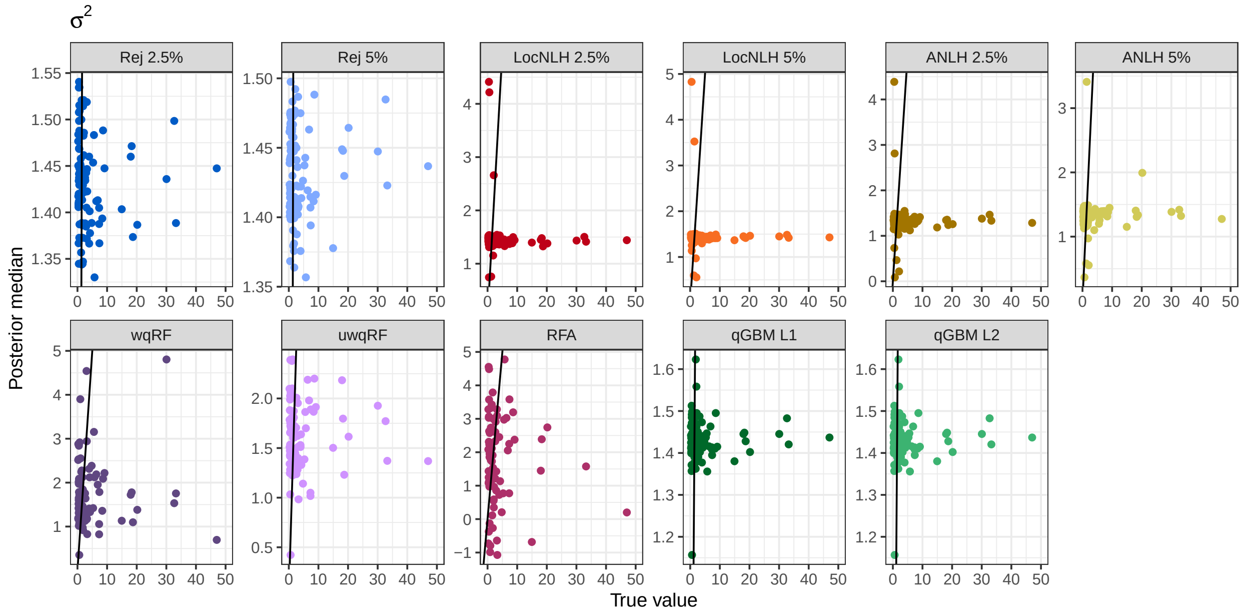


(h) $\sigma^2$

Figure 2: *ABC posterior median as a function of the true parameter value (cont.). 'Rej': rejection ABC algorithm, 'LocNLH': local nonlinear heteroscedastic regression, 'ANLH': adaptive nonlinear heteroscedastic regression, 'RFA': adjusted random forest regression, 'wqRF' (resp; 'uwqRF') : weighted (resp. unweighted) quantile regression via random forests, 'qGBM L1' (resp; 'qGBM L2'): quantile regression via gradient boosting and $L_1$ (resp. $L_2$) loss. The percentages '2.5%' and '5%' correspond to the values of the threshold parameter $\varepsilon$*

## 2 Real data study

Table 2 gives the posterior median and 95% credible interval for each parameter, obtained with all the methods.

Table 2: *Posterior median and 95% CI for each parameter and each method, on the real dataset. 'Rej': rejection ABC algorithm, 'LocNLH': local nonlinear heteroscedastic regression, 'ANLH': adaptive nonlinear heteroscedastic regression, 'RFA': adjusted random forest regression, 'wqRF' (resp; 'uwqRF') : weighted (resp. unweighted) quantile regression via random forests, 'qGBM L1' (resp; 'qGBM L2'): quantile regression via gradient boosting and $L_1$ (resp. $L_2$) loss. The percentages '2.5%' and '5%' correspond to the values of the threshold parameter $\varepsilon$*

| Method | $\tau_0$ | $f_0$ | $a$ | $b$ |
|---|---|---|---|---|
| Rej 2.5% | 516.9 [112.4 ; 966.3] | 0.101 [0.015 ; 0.716] | 500.1 [26.6 ; 974.7] | 491.6 [22.5 ; 970.6] |
| Rej 5% | 530.0 [110.5 ; 970.7] | 0.102 [0.015 ; 0.709] | 508.7 [29.2 ; 975.7] | 489.6 [20.5 ; 971.3] |
| LocNLH 2.5% | 571.3 [241.0 ; 942.9] | 0.102 [0.015 ; 0.718] | 560.6 [100.1 ; 981.7] | 226.3 [100.0 ; 853.2] |
| LocNLH 5% | 691.9 [345.2 ; 968.8] | 0.104 [0.015 ; 0.714] | 618.9 [100.0 ; 985.2] | 411.8 [100.0 ; 951.1] |
| ANLH 2.5% | 582.6 [345.0 ; 832.5] | 0.097 [0.013 ; 0.386] | 495.8 [100.1 ; 955.5] | 203.4 [100.0 ; 460.4] |
| ANLH 5% | 685.3 [461.2 ; 913.6] | 0.099 [0.015 ; 0.382] | 581.9 [100.1 ; 973.5] | 351.4 [100.0 ; 841.5] |
| wqRF | 669.0 [329.2 ; 982.2] | 0.295 [0.024 ; 1.326] | 609.7 [82.9 ; 991.0] | 427.7 [14.7 ; 981.4] |
| uwqRF | 660.5 [317.4 ; 982.5] | 0.172 [0.017 ; 1.467] | 573.7 [39.5 ; 975.4] | 430.5 [12.4 ; 965.8] |
| RFA | 560.4 [352.3 ; 837.0] | 0.270 [0.140 ; 0.880] | 511.8 [61.4 ; 1005] | 491.2 [19.89 ; 969.8] |
| qGBM L1 | 548.0 [113.8 ; 971.6] | 0.102 [0.015 ; 0.719] | 513.0 [29.2 ; 975.8] | 482.8 [20.7 ; 971.9] |
| qGBM L2 | 548.0 [113.8 ; 971.6] | 0.102 [0.015 ; 0.719] | 513.0 [29.2 ; 975.8] | 482.8 [20.7 ; 971.9] |
| Method | $\beta_1$ | $\beta_2$ | $\beta_3$ | $\sigma^2$ |
| Rej 2.5% | 0.773 [-11.10 ; 7.240] | -1.654 [-20.6 ; 10.56] | 8.497 [2.493 ; 20.289] | 1.413 [0.261 ; 29.46] |
| Rej 5% | 0.331 [-11.63 ; 7.653] | -2.536 [-20.28 ; 10.53] | 8.154 [1.619 ; 20.08] | 1.414 [0.257 ; 32.49] |
| LocNLH 2.5% | 0.909 [-12.13 ; 6.470] | 0.631 [-17.36 ; 10.35] | 8.281 [3.573 ; 20.83] | 1.498 [0.282 ; 29.92] |
| LocNLH 5% | 0.841 [-11.91 ; 5.950] | 3.051 [-12.39 ; 12.12] | 7.590 [3.359 ; 20.35] | 1.440 [0.262 ; 33.62] |
| ANLH 2.5% | 3.888 [-1.349 ; 7.333] | 1.653 [-6.338 ; 5.677] | 5.439 [2.685 ; 10.43] | 1.441 [0.293 ; 17.12] |
| ANLH 5% | 1.930 [-3.117 ; 5.060] | 3.218 [-6.725 ; 9.045] | 6.999 [4.566 ; 11.71] | 1.336 [0.259 ; 16.47] |
| wqRF | 4.182 [-8.146 ; 10.80] | 1.424 [-0.321 ; 3.414] | 5.140 [4.087 ; 6.375] | 7.724 [0.380 ; 262.1] |
| uwqRF | 4.398 [-6.459 ; 9.551] | 1.424 [-2.407 ; 8.282] | 5.191 [2.118 ; 7.393] | 3.285 [0.314 ; 261.5] |
| RFA | 3.497 [-3.850 ; 8.379] | 1.483 [-11.52 ; 10.85] | 4.89 [1.070 ; 11.63] | 56.17 [45.13 ; 84.86] |
| qGBM L1 | 0.648 [-10.73 ; 7.598] | -2.012 [-18.87 ; 10.64] | 7.825 [1.690 ; 19.10] | 1.421 [0.257 ; 33.73] |
| qGBM L2 | 0.648 [-10.73 ; 7.598] | -2.012 [-18.87 ; 10.64] | 7.825 [1.690 ; 19.10] | 1.421 [0.257 ; 33.73] |

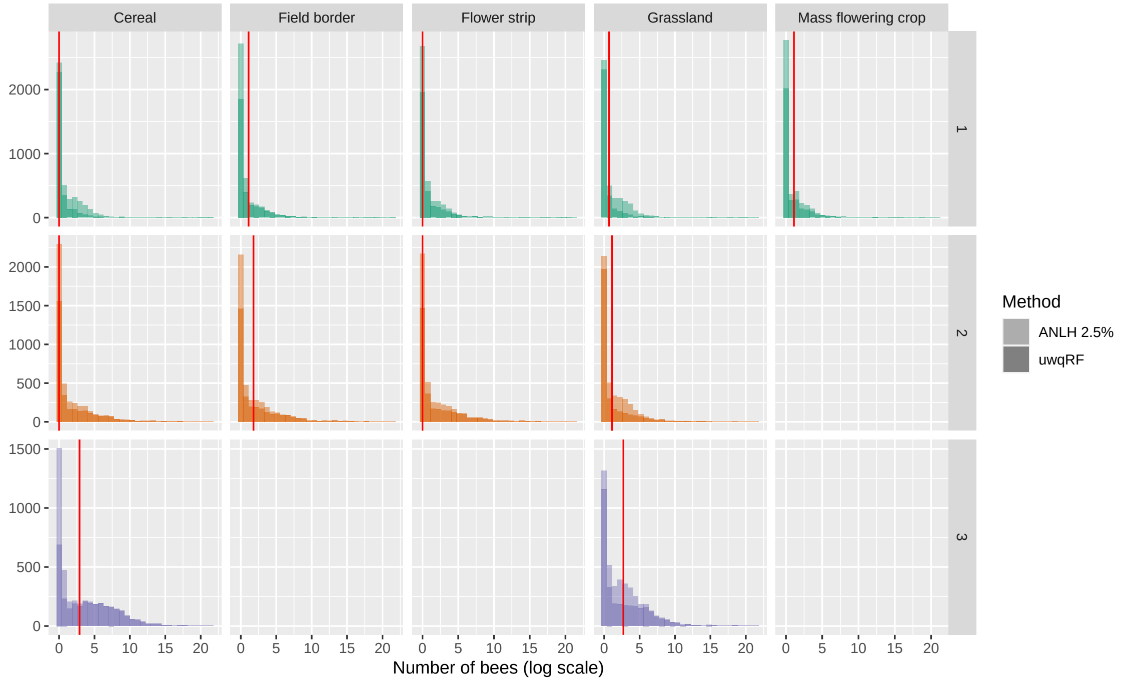


Figure 3: *Distribution of predicted values for 11 randomly selected datapoints covering each landuse and period, for ANLH ($\varepsilon = 2.5\%$) and uwqRF approaches.*

Figure 3 compares the distribution of predicted values obtained with quantile regression via unweighted random forests and adaptive nonlinear local regression, for 11 randomly selected sampling locations. The red vertical line indicates the value of the observed number of bee at the correspond sampling points.

Figure 4 gives the distribution of the projection of the predicted summary statistics on the second and third axes of a principal component analysis performed on the ABC table (i.e. the principal components are obtained from a PCA based on the summary statistics of the ABC table, and then the coordinates of the predicted summary statistics along each principal axis are computed).

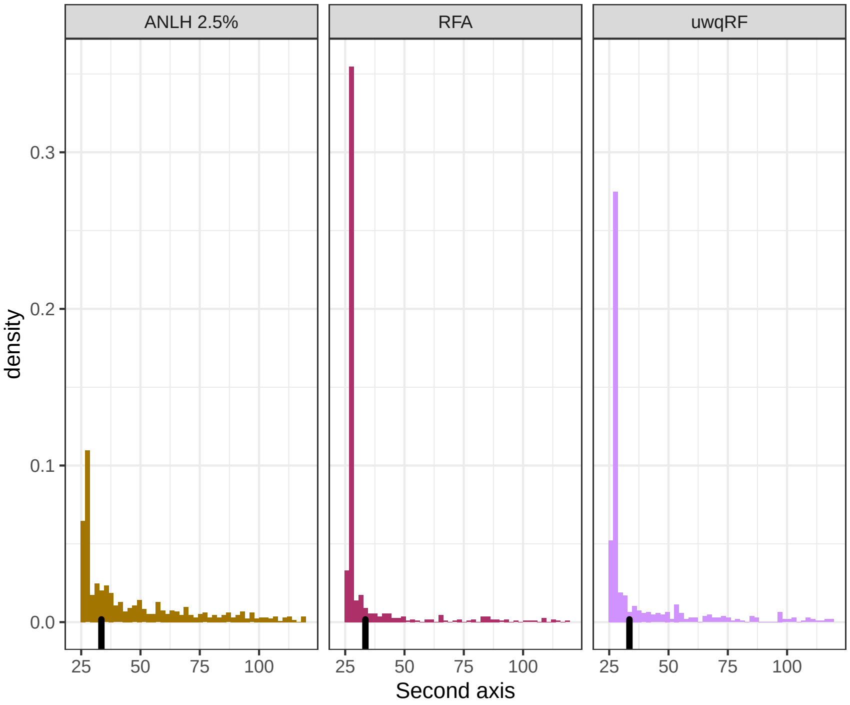


(a) *Second axis*

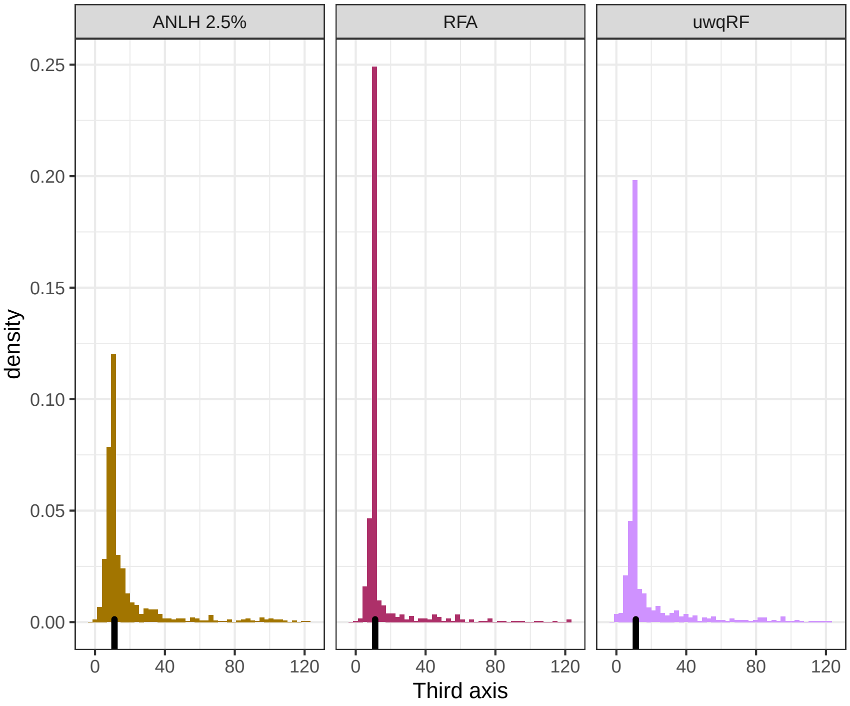


(b) *Second axis*

Figure 4: *Histogram of the summary statistics along the second and third axis of the PCA (left panel: adaptive nonlinear local regression (ANLH), middle panel: nonlinear regression via random forests (RFA) and right panel: quantile regression via unweighted random forests. The black segments correspond to the location of the observed summary statistics on the first PCA axis.*
